# Supplementary material for: Finding the Missing-half: Graph Complementary Learning for Homophily-prone and Heterophily-prone Graphs
Source: arXiv:2306.07608 source file (2023-06-13)
Supplement: Supplementary file 1 [file Appendix_filters.tex]

\begin{figure}[h]
    \centering
\includegraphics[scale = 0.5]{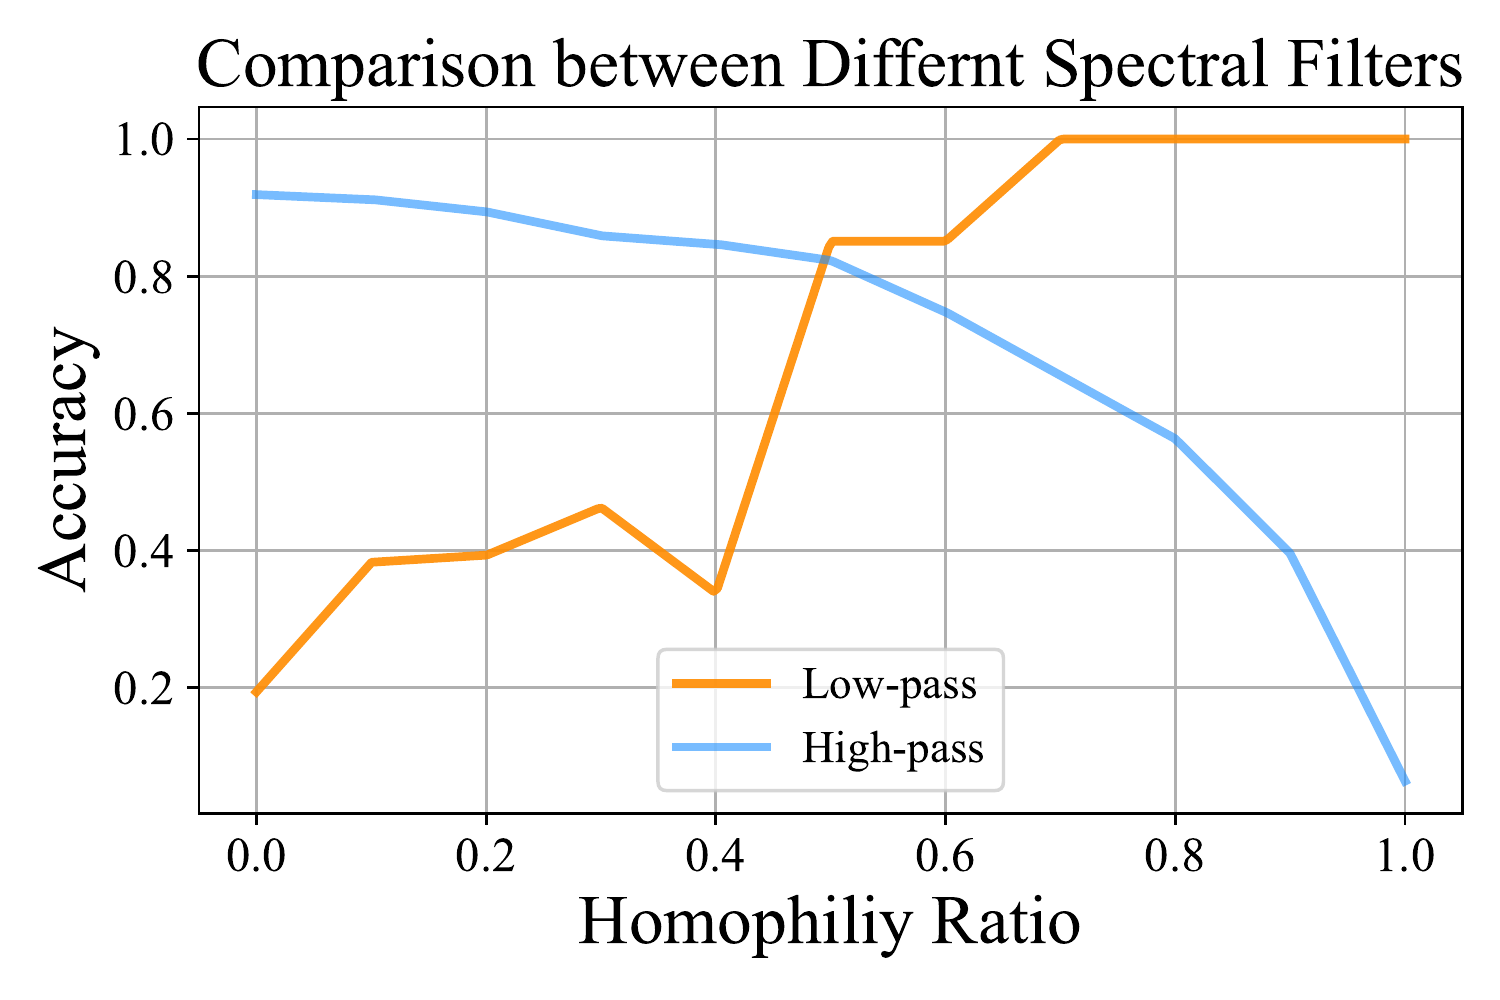}
    \caption{Comparison between Different Spectral Filters on a synthetic dataset.}
    \label{fig:compare different filters}
\end{figure}
To validate our finding in section~\ref{sec:explore}, we conduct experiments for the four spectral filters (i.e., low-pass, high-pass, band-pass, and band-reject) on synthetic datasets. The synthetic datasets are built based on the Cora dataset. Specifically, we delete all the edges in the Cora dataset and add synthetic connections to it. These connections have a homophily ratio ranging from 0 to 1. The definition of homophily ratio is provided in Definition~\ref{def:homo ratio}.

From Figure~\ref{fig:compare different filters} above, we can observe that the experiment result is consistent with our findings in section~\ref{sec:explore}. When increasing the homophily ratio, the performance of High-pass and Band-pass filters is generally on the decline, whereas Low-pass and Band-reject are on the rise. Accordingly, high-pass and band-pass filters perform well when a graph has a low homophily ratio. Low-pass and band-reject filters, on the other hand, prefer graphs with a high homophily ratio.
