# Supplementary material for: Finding the Missing-half: Graph Complementary Learning for Homophily-prone and Heterophily-prone Graphs
Source: arXiv:2306.07608 source file (2023-06-13)
Supplement: Supplementary file 2 [file Appendix_fourthterm.tex]

We propose the following proposition to show this point:
\begin{proposition}
For \rm $\textbf{H}^{l + 1} = \sigma(-\hat{\textbf{A}}_{homo}\hat{\textbf{A}}_{heter}\textbf{H}^l\textbf{W}^l$, ignoring the effect of $\textbf{W}^{l})$ and the non-linearity $\sigma(\cdot)$ in each layer, its optimisation objective is:
\end{proposition}
\begin{align}
    \begin{aligned}
        \mathcal{O}_{conv} &= \underset{\textbf{H}}{min}\{\textbf{H}^T\hat{\textbf{A}}_{homo}\hat{\textbf{A}}_{heter}\textbf{H}\}, \\ &= \sum^{D'}_k(\textbf{H}^T\hat{\textbf{A}}_{homo})(\hat{\textbf{A}}_{heter}\textbf{H})[{:,k}]),
    \end{aligned}
    \label{eq:conv obj}
\end{align}
\begin{proof}
Following the assumption that both $\hat{\textbf{A}}_{homo}$ and $\hat{\textbf{A}}_{heter}$ are non-bipartite and connected, we can know $\hat{\textbf{A}}_{homo}\hat{\textbf{A}}_{heter}$ is still positive semi-definite. Thus, we can solve the objective above via $\frac{\partial tr(\textbf{H}\hat{\textbf{A}}_{homo}\hat{\textbf{A}}_{heter}\textbf{H})}{\partial \textbf{H}} = 0$:
\begin{align}
    \begin{aligned}
\hat{\textbf{A}}_{homo}\hat{\textbf{A}}_{heter}\textbf{H} = 0 &\to -\hat{\textbf{A}}_{homo}\hat{\textbf{A}}_{heter}\textbf{H} = 0 , \\ &\to (\textbf{I} -  \hat{\textbf{A}}_{homo}\hat{\textbf{A}}_{heter}) \textbf{H} = \textbf{H}.
    \end{aligned}
\end{align}
\end{proof}
The derived formula is consistent with the one in the proposition and thus we prove it.
