# Supplementary material for: Finding the Missing-half: Graph Complementary Learning for Homophily-prone and Heterophily-prone Graphs
Source: arXiv:2306.07608 source file (2023-06-13)
Supplement: Supplementary file 3 [file Appendix_heterophilic_dominant.tex]

Given a dataset $\textbf{X} \in \mathbb{R}^{N \times D}$ with $C$ classes and assuming these classes are evenly distributed, it is easy to deduce that homophilic node pairs have $C(\frac{N}{C})^2$. In contrast, the number of heterophilic node pairs is $N^2 - C(\frac{N}{C})^2$. Then the formula for calculating the ratio of homophilic node pairs in a dataset can be defined as follows:
\begin{equation}
    \mathcal{M}(\mathcal{G}) = \frac{C(\frac{N}{C})^2}{N^2} \to \frac{1}{C},
\end{equation} 
where $\mathcal{M}(\cdot)$ is the function to calculate the ratio given a graph $\mathcal{G}$. Here we can see when $C$ increases, the ratio plummets. In particular, we can see when $C > 2$, which is very common in real-world datasets, heterophilic node pairs would be dominant in a dataset. Thus, heterophilic-prone node pairs would have a similar distribution to randomly sampled node pairs in terms of cosine similarity.
